# Supplementary material for: Zodiacal Exoplanets in Time (ZEIT) V: A Uniform Search for Transiting Planets in Young Clusters Observed by K2
Source: arXiv:1709.09670 source file (2017-09-29)
Supplement: Supplementary file 1 [file supptables.tex]

\documentclass[onecolumn]{aastex6}
\usepackage{aas_macros}
\usepackage{amsfonts}
\usepackage{amsmath}
\usepackage{graphicx}
\usepackage{subfigure}

%%All the membership tables

%ApJ following 2 lines
\shorttitle{ZEIT V}
\shortauthors{Rizzuto et al.}
%ApJ 
\begin{document}
\title{Zodiacal Exoplanets in Time (ZEIT) V: Limits on Additional Transiting Exoplanets in the ZEIT Systems.} % AWM since the main part of this paper is the search algorithm you might highlight it in the title 

%%TODO:
% -Full transit search results, including inspection of outputs that already exist and rerunning on small subset of fast rotators in 0.5 mode
% -Eccentricity effects plots. The data for these exists but nicer plots can be remade.
% -Extra planet limits plots, clean them up, maybe rerun these with newer code
% -Explanation of any candidates that aren't real.

\author{
Aaron C. Rizzuto\altaffilmark{1},
Andrew W. Mann\altaffilmark{1},
Andrew  Vanderburg\altaffilmark{2},
Adam L. Kraus\altaffilmark{1}
}

\altaffiltext{1}{Department of Astronomy, The University of Texas at Austin, Austin, TX 78712, USA}
\altaffiltext{2}{HarvardÐSmithsonian Center for Astrophysics, 60 Garden St., Cambridge, MA 02138, USA}

\section{Online Tables}
%%This needs to be supplementary materials, then uploaded to vizier, it's ~80 pages

% [inline block 0: 5 envs, 488984 chars -> data_tex | \begin{deluxetable}{ccccccccccccc}  \tabletypesize{\scriptsize} ...]


\end{document}
